# Supplementary material for: Learning Attribute-Structure Co-Evolutions in Dynamic Graphs
Source: arXiv:2007.13004 source file (2020-07-25)
Supplement: Supplementary file 1 [file 8appendix.tex]

\section{Reproducibility Justification}
This section provides a justification of the proposed method's reproducibility, covering information necessary for reproducing the experimental results, insights, or conclusions reported in the paper.

\subsection{Datasets}
We used 4 datasets from two type of evolutionary graphs. \\
\noindent \textbf{Evolutionary co-authorship graph}. 
We built a sequence of yearly co-authorship graphs by collecting $226,611$ papers from 2001 to 2010 in computer science from Microsoft Academic Graph \cite{wang2020microsoft}. Authors were ranked by their number of papers. The top $2,000$ and $10,000$ were used to make two datasets denoted by $\mathcal{D}_{\textsc{au}}^{2K}$ and $\mathcal{D}_{\textsc{au}}^{10K}$. The venues and the paper title's words were used as node attributes after filtering out infrequent ones. As a result, we have $316$ venues and $3,549$ words in $\mathcal{D}_{\textsc{au}}^{2K}$; and $448$ venues, $6,442$ words in $\mathcal{D}_{\textsc{au}}^{10K}$.\\
\noindent \textbf{Evolutionary virtual currency graph}.
We used 2 benchmark datasets \text{Bitcoin-OTC} and \text{Bitcoin-Alpha} of Bitcoin transaction networks \cite{kumar2018rev2} denoted by $\mathcal{D}_{\textsc{bc}}^{\text{otc}}$ and $\mathcal{D}_{\textsc{bc}}^{\text{alp}}$. We followed the treatments as in \cite{pareja2019evolvegcn} to form a sequence of graphs with 138 time steps (each for about 2 weeks), and use node in/out degree as input features.

\subsection{Parameter Settings}
%Our \textsc{CalendarGNN} (and \textsc{CalendarGNN-Attn}) was implemented in \text{PyTorch} \cite{paszke2017automatic}. We use {Stochastic Gradient Descent} \cite{bottou2010large} and {AMDM} \cite{kingma2014adam} updating rule with initial learning rate $\alpha=10^{-4}$ for training.
%We set the dimensions as 256 for session embeddings (i.e., $K_\mathcal{S}$) and all spatial/temporal unit embeddings, (i.e., $K_h$, $K_w$, $K_y$, and $K_l$). And, the dimensions for all spatial/temporal patterns (i.e., $K_{\mathcal{T}_h}$, $K_{\mathcal{T}_w}$, $K_{\mathcal{T}_y}$, and $K_{\mathcal{L}}$) are set as 128. The dimensions of user final representation $K_{\mathcal{U}}$ is $512=128\times 4$ for \textsc{CalendarGNN}, and equals $768=(128+128)\times 3$ for \textsc{CalendarGNN-Attn}. Besides, due to anonymization, the features for items nodes $\mathcal{V}$ and locations nodes $\mathcal{L}$ provided in the above open datasets only include the identification information.
We use open-source implementations provided by the original paper for all baseline methods.
For \textsc{GraphSAGE} and \textsc{EvolveGCN}, we compute $\mathbf{H}^{t_{test}} \cdot \left( \mathbf{H}^{t_{train}\,\rm{T}} \cdot \mathbf{X}^{t_{train}} \right)$ as their attribute inference matrix. The last node embeddings matrix $\mathbf{H}^{t_{test}-1}$ from training graph snapshots and the last training attribute matrix $\mathbf{X}^{t_{test}-1}$ are treated as $\mathbf{H}^{t_{train}}$ and $\mathbf{X}^{t_{train}}$ for \textsc{EvolveGCN}.
The core hyper-parameters of all baselines are set following the recommendations from their inventors or otherwise selected using the grid search strategy: $\beta_{0}$ and $\beta_{1}$ of \textsc{DynamicTriad} are found in $\{ 0.01, 0.1, 1, 10\}$; $w_{n}$ of \textsc{DySAT} is found in $\{0.01, 0.1, 1\}$; the number of recurrent layers for \textsc{DCRNN} and the number of spatio-temporal convolutional blocks for \textsc{STGCN} are found in $\{1, 2\}$.
All deep models are trained by a maximum of $100$ epochs. The embedding size is $256$ for $\mathcal{D}_{\textsc{au}}^{10K}$ and $512$ in other cases.

\subsection{Evaluation Metrics}
For {node attribute prediction}, we use Mean Average Error (MAE) and Root Mean Squared Error (RMSE); for {link prediction}, we use Area Under the precision-recall Curve (AUC), F1 measure, and Precision@$50,100,200$. Because the raw attributes were very sparse in $\mathcal{D}_{\textsc{au}}^{2K}$ and $\mathcal{D}_{\textsc{au}}^{10K}$, for all methods, we subsample the same number of close-to-zero predictions as the number of bigger-than-1 predictions during test to make it comparable.

\section{Algorithms}
\subsection{Framework}
The pseudocode of the \textsc{CoEvoGNN} is shown in Algorithm \ref{alg:framework}.

\begin{algorithm}[t]
	\SetAlgoLined
	\SetKwInOut{Input}{Input}
	\SetKwInOut{Output}{Output}
	\Input{Dynamic graph sequence $\{(G^t, \mathbf{X}^t) \,|\, t=0,\dots,T \}$; parameter matrices $\{\mathbf{W}^{\langle s \rangle} \,|\, s=1,\dots,S \}$ and fusion matrix $\mathbf{\Gamma}$; temporal evolution span $S$; and, static graph neural models $\{f_{static}^{\langle s \rangle} \,|\, s=1,\dots,S \}$.}
	\Output{Node latent embeddings $\mathbf{h}_{v}^{t}$, $v \in \mathcal{V}$ and $1 \leq t \leq T$.}
	\For{$v \in \mathcal{V}$}{
	// Initialization \\
	$\mathbf{h}_{v}^{0} \leftarrow f_{static}^{\langle 1 \rangle}(v \,|\, ({G}^0, \mathbf{X}^{0}), 1)$ \\
		\For{$t=1,\dots,T$}{
			// Structural aggregations \\
			Let $\hat{H}_v[1,\dots,\min{(t,S)}]$ and $E_v[1,\dots,\min{(t,S)}]$ be new arrays \\
			\For{$s=1,\dots,\min{(t,S)}$}{
				$\hat{\mathbf{h}}_{v}^{\! \langle s \rangle} \leftarrow f_{static}^{\langle s \rangle}(v \,|\, ({G}^{t-s}, \mathbf{X}^{t-s}), L)$ \\
				$e_{v}^{\! \langle s \rangle} \leftarrow {(\mathbf{h}_{v}^{t-s})}^\top \cdot \mathbf{\Gamma} \cdot \hat{\mathbf{h}}_{v}^{\! \langle s \rangle}$ \\
				$\hat{H}_v[s] = \hat{\mathbf{h}}_{v}^{\! \langle s \rangle}$ and $E_v[s] = e_{v}^{\! \langle s \rangle}$ \\
			}
			// Temporal self-attention \\
			Let $A_v[1,\dots,\min{(t,S)}]$ be a new array \\
			\For{$s=1,\dots,\min{(t,S)}$}{
				$a_{v}^{\! \langle s \rangle} \leftarrow \frac{\exp{(E_v[s])}}{\sum_{s'=1}^{\min{(t,S)}} \exp{(E_v[s'])}}$ \\
				$A_v[s] = a_{v}^{\! \langle s \rangle}$ \\
			}
			// Fusion and normalization \\
			$\mathbf{h}_{v}^{t} \leftarrow \sum_{s=1}^{\min{(t,S)}} A_v[s] \, \sigma \left( \mathbf{W}^{\langle s \rangle} \cdot \left[ \mathbf{h}_{v}^{t-s}; \hat{H}_v[s] \right] \right)$ \\
			$\mathbf{h}_{v}^{t} \leftarrow \mathbf{h}_{v}^{t} / {\left\| \mathbf{h}_{v}^{t} \right\|}_{2}$ \\
		}
	}
	\caption{\textsc{CoEvoGNN} framework}
	\label{alg:framework}
\end{algorithm}

\begin{algorithm}[t]
	\SetAlgoLined
	Initialize model parameters $\{\mathbf{W}^{\langle s \rangle} \,|\, s=1,\dots,S \}$, $\mathbf{\Gamma}$, and $\mathbf{M}$ \\
	\Repeat{finish}{
		Sample minibatch of nodes $\mathcal{V'}$ from all nodes $\mathcal{V}$ \\
 		// Generate evolutionary embeddings \\
		$\mathbf{H}^1,\dots,\mathbf{H}^T \leftarrow \textsc{CoEvoGNN}(\mathcal{V'})$ \Comment{see Algorithm \ref{alg:framework}}\\
		// Compute evolutionary losses \\
		$\mathcal{J}_{\mathbf{X}^{1}},\dots,\mathcal{J}_{\mathbf{X}^{T}} \leftarrow$ Compute the attribute evolutionary loss for attribute inference \Comment{see Equation (\ref{eqn:loss_attribute})}\\
		$\mathcal{J}_{{G}^{1}},\dots,\mathcal{J}_{{G}^{T}} \leftarrow$ Compute the structure evolutionary loss for link prediction \Comment{see Equation (\ref{eqn:loss_structure})}\\
		$\mathcal{J} \leftarrow$ Compute overall loss \Comment{see Equation (\ref{eqn:loss_overall})}\\
		// Update parameters \\
		$\mathbf{W}^{\langle \cdot \rangle} \stackrel{+}\leftarrow - \nabla_{\mathbf{W}^{\langle \cdot \rangle}}(\mathcal{J})$\\
		$\mathbf{\Gamma} \stackrel{+}\leftarrow - \nabla_{\mathbf{\Gamma}}(\mathcal{J})$\\
		$\mathbf{M} \stackrel{+}\leftarrow - \nabla_{\mathbf{M}}(\mathcal{J})$\\
	}
	\caption{Training procedure of \textsc{CoEvoGNN}}
	\label{alg:training}
\end{algorithm}

\subsection{The training}
The training procedures of \textsc{CoEvoGNN} is shown in Algorithm \ref{alg:training}.

\section{Additional Experimental Results}
This section provides more experimental results not fully covered in Section \ref{sec:experiments} for validating the effectiveness of the proposed method.

\subsection{Effect of $S$-stack temporal self-attention}
To understand \textsc{CoEvoGNN}'s advantage, we further examine the effectiveness of the $S$-stack temporal self-attention architecture which is the core component for distilling and fusing influence from multiple previous graph snapshots. In particular, we examine different choices of the temporal evolution span $S$, and conduct ablation studies to verify the contribution of temporal self-attention.

\subsubsection{Choice of temporal evolution span $S$}
\label{subsubsec:architecture_s}
\textsc{CoEvoGNN} is designed to fuse the influence from multiple previous graph snapshots and the temporal evolution span hyperparameter $S$ controls how many previous snapshots to be fused at each time step. On one hand, setting $S=1$ enforces \textsc{CoEvoGNN} to follow the Markov property \cite{aggarwal2014evolutionary} and generate new node embedding relying only on the previous one. This would largely limit \textsc{CoEvoGNN}'s expressive power on the co-evolution pattern. On the other hand, setting $S$ to a large value brings in additional computational burden since real evolutionary graph exhibits a time decay effect (see Section \ref{sec:motivation}). We test different values of $S$ up to $8$ and present the results in Table \ref{tab:architecture_s} and Figure \ref{fig:architecture_s}.

For evolutionary co-authorship graphs $\mathcal{D}_{\textsc{au}}^{2K}$ and $\mathcal{D}_{\textsc{au}}^{10K}$, increasing the value of $S$ from $1$ up to $3$ can make \textsc{CoEvoGNN} achieving better performance on both tasks: the RMSE decreases from $0.988$ to $0.938$ on $\mathcal{D}_{\textsc{au}}^{2K}$ (from $0.897$ to $0.828$ on $\mathcal{D}_{\textsc{au}}^{10K}$) for future node attribute prediction; and the F1 improves from $0.236$ to $0.274$ on $\mathcal{D}_{\textsc{au}}^{2K}$ (from $0.149$ to $0.170$ on $\mathcal{D}_{\textsc{au}}^{10K}$) for future graph link prediction.
After that, further increasing $S$ brings little improvement and the performance slightly drops at $S=8$ probably due to too much noise. 
The similar trend can also be observed on evolutionary virtual currency graphs $\mathcal{D}_{\textsc{bc}}^{\text{otc}}$ and $\mathcal{D}_{\textsc{bc}}^{\text{alp}}$ and the diminishing marginal benefits of increasing $S$ are noticeable. But different from co-authorship graphs, the elbow point appears at $S=5$. This can be explained by the fact that these two virtual currency graphs contains longer time steps ($138$ vs. $10$ of $\mathcal{D}_{\textsc{au}}^{2K}$ and $\mathcal{D}_{\textsc{au}}^{10K}$) and each graph is also sparser. So, \textsc{CoEvoGNN} needs longer historical information in generating each new node embedding. In practice, we suggest using a grid search strategy to find the optimal $S$ value in the range of $[2, 8]$.

\begin{figure}[t]
    \centering
    \subfigure[Node attribute prediction. Lower RMSE indicates better performance.]
    {\includegraphics[width=0.48\linewidth]{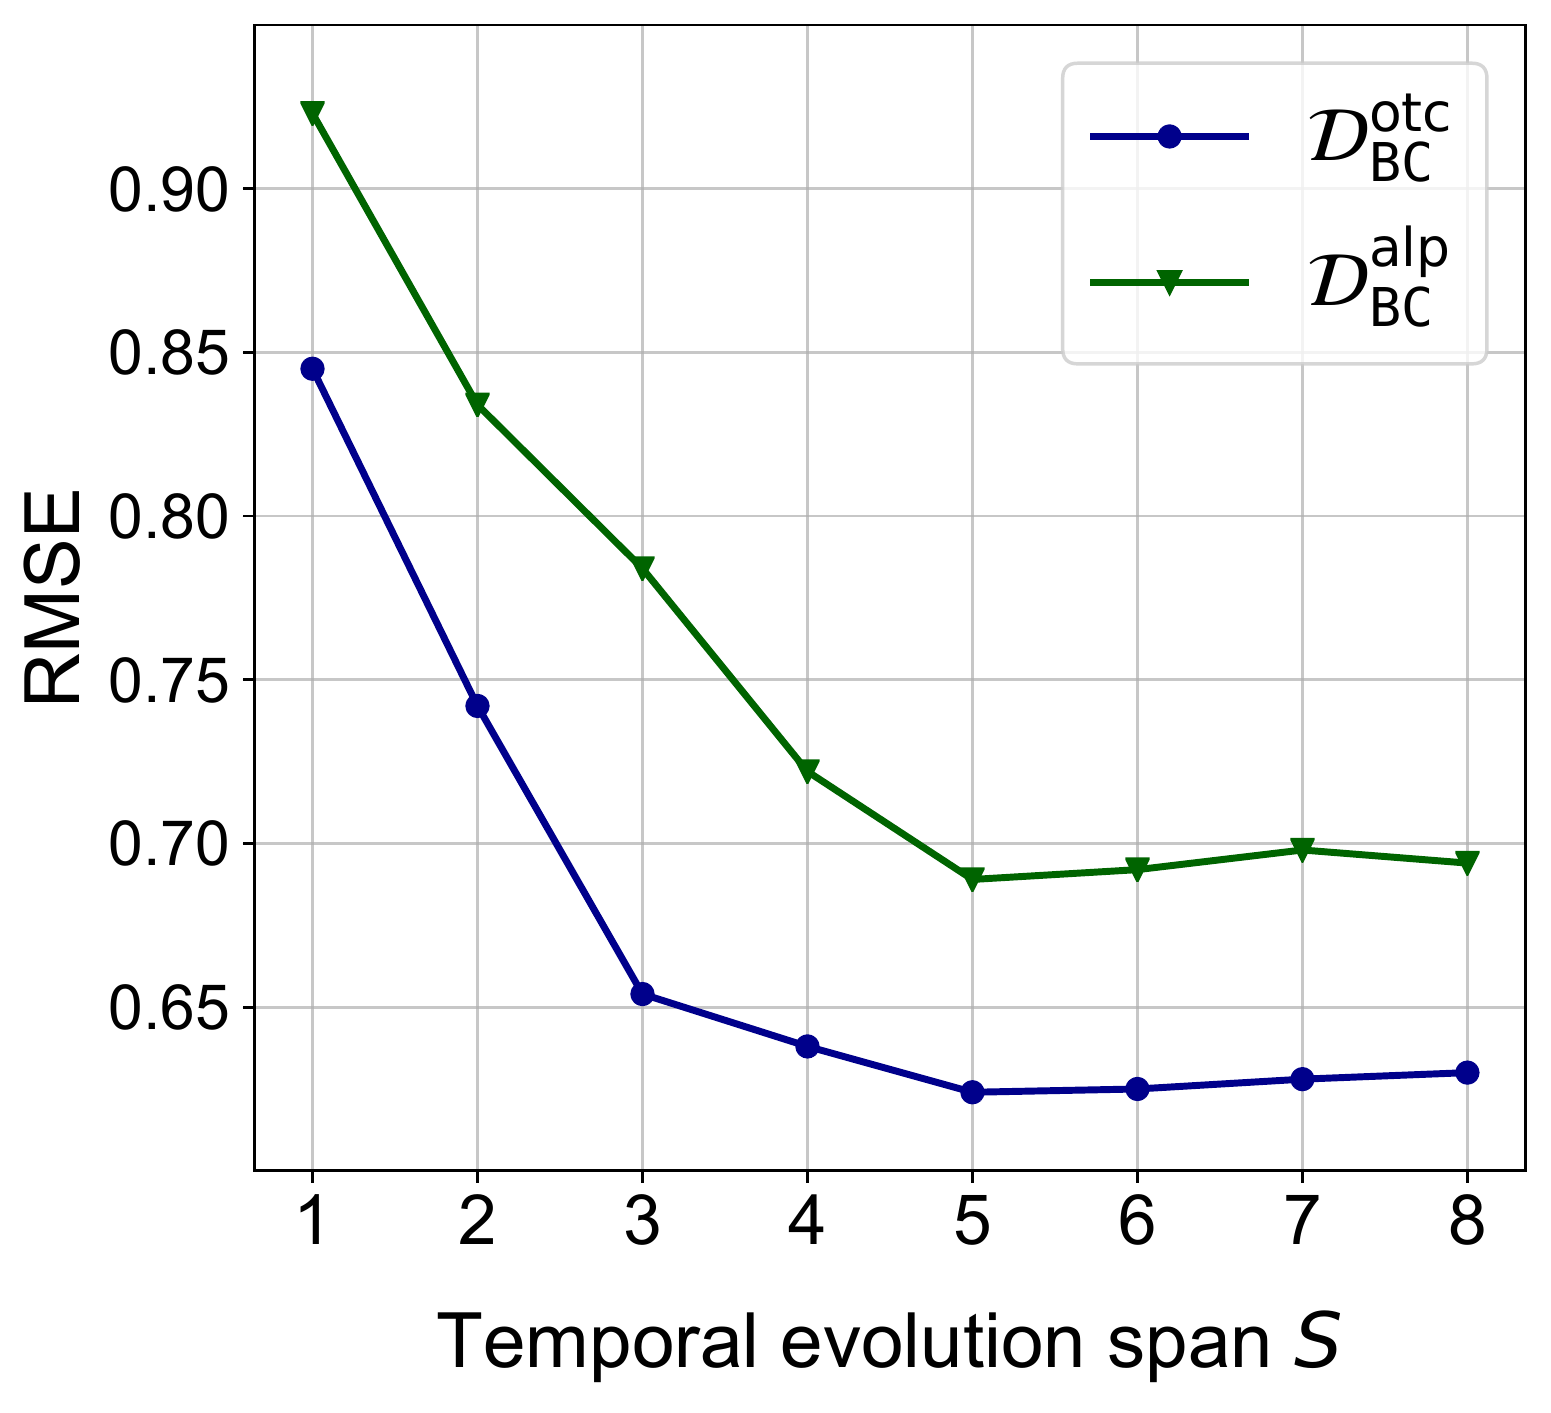}\label{fig:architecture_s_1}}
    \hfill
    \subfigure[Graph link prediction. Higher F1 indicates better performance.]
    {\includegraphics[width=0.48\linewidth]{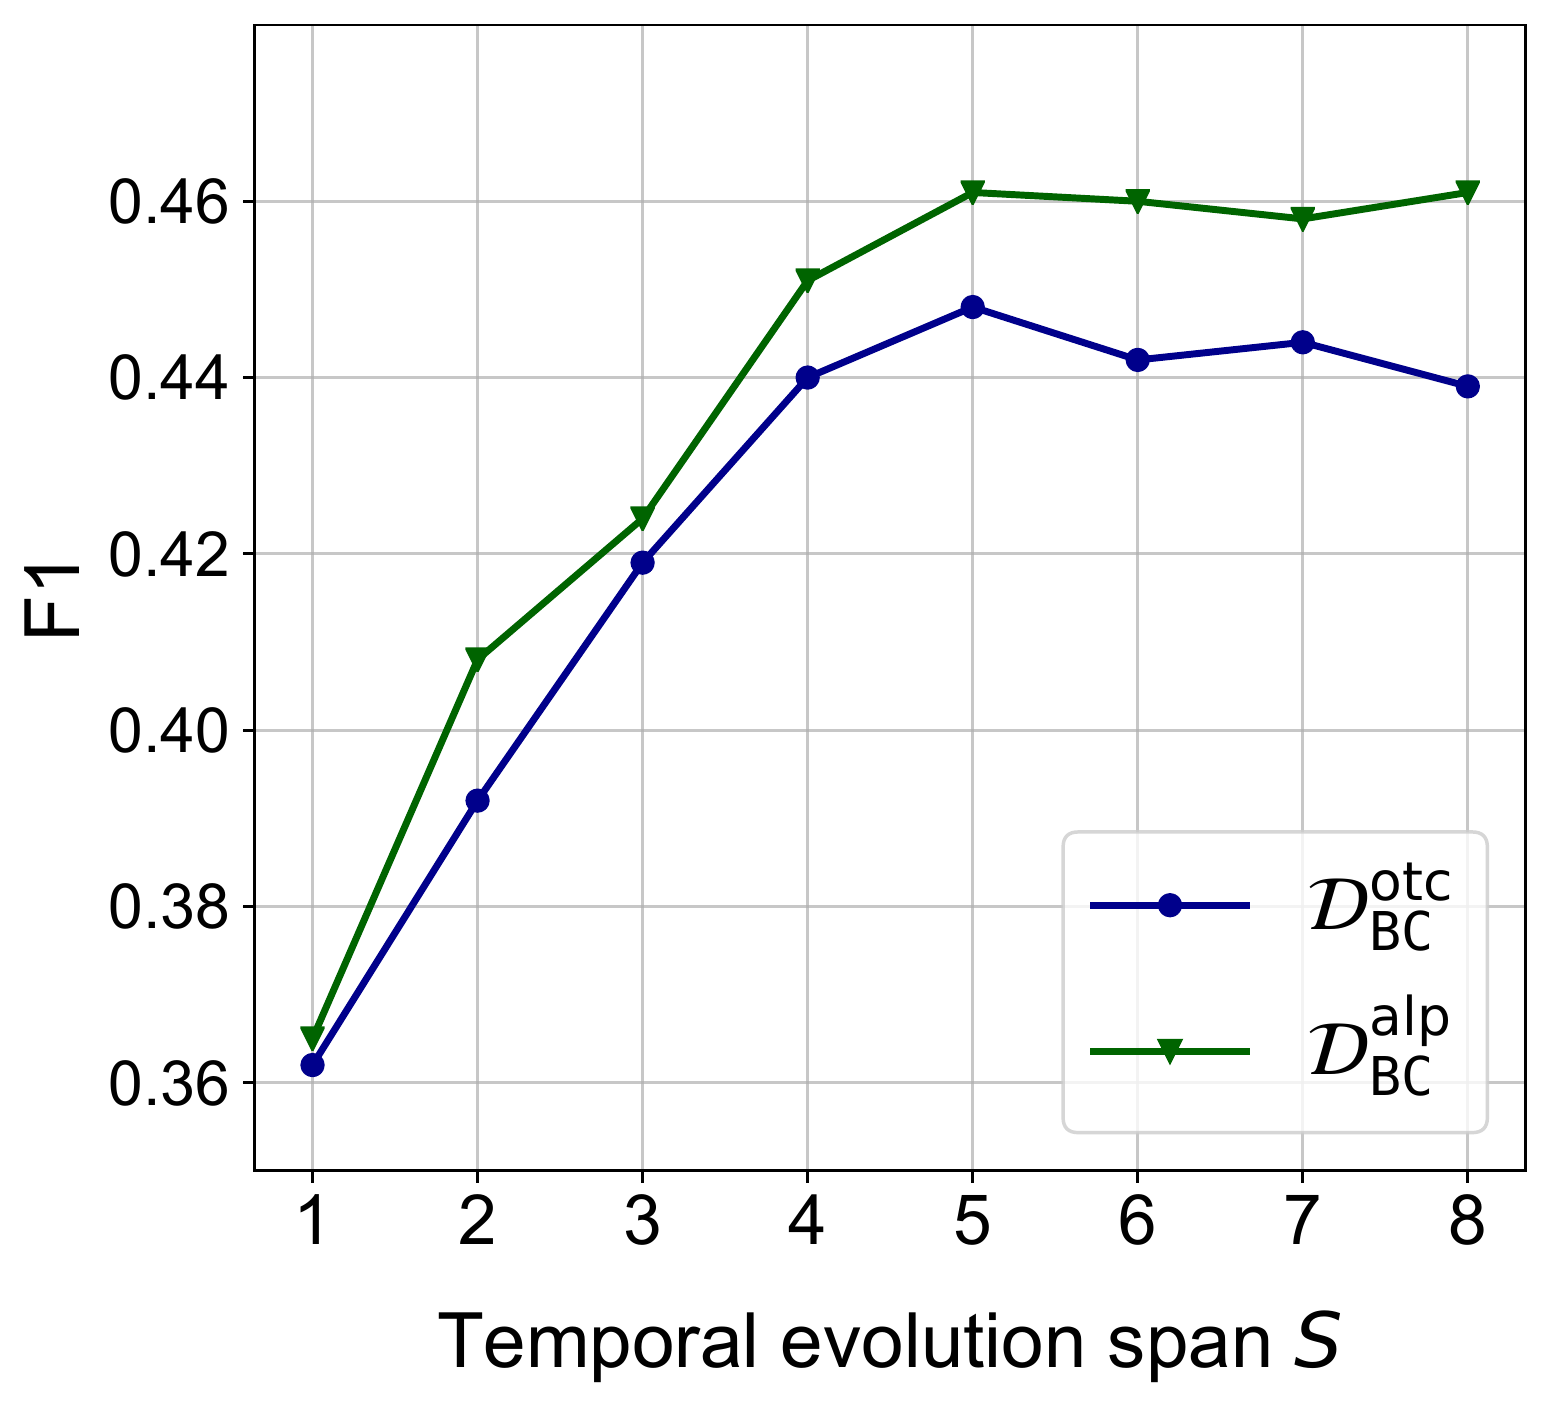}\label{fig:architecture_s_2}}
	\vspace{-0.2in}
    \caption{Forecasting node attributes and links in bitcoin graphs with different values of temporal evolution span $S$.}
    \label{fig:architecture_s}
    \vspace{-0.2in}
\end{figure}

\begin{figure}[t]
    \centering
    \subfigure[Node attribute prediction. Lower RMSE indicates better performance.]
    {\includegraphics[width=0.48\linewidth]{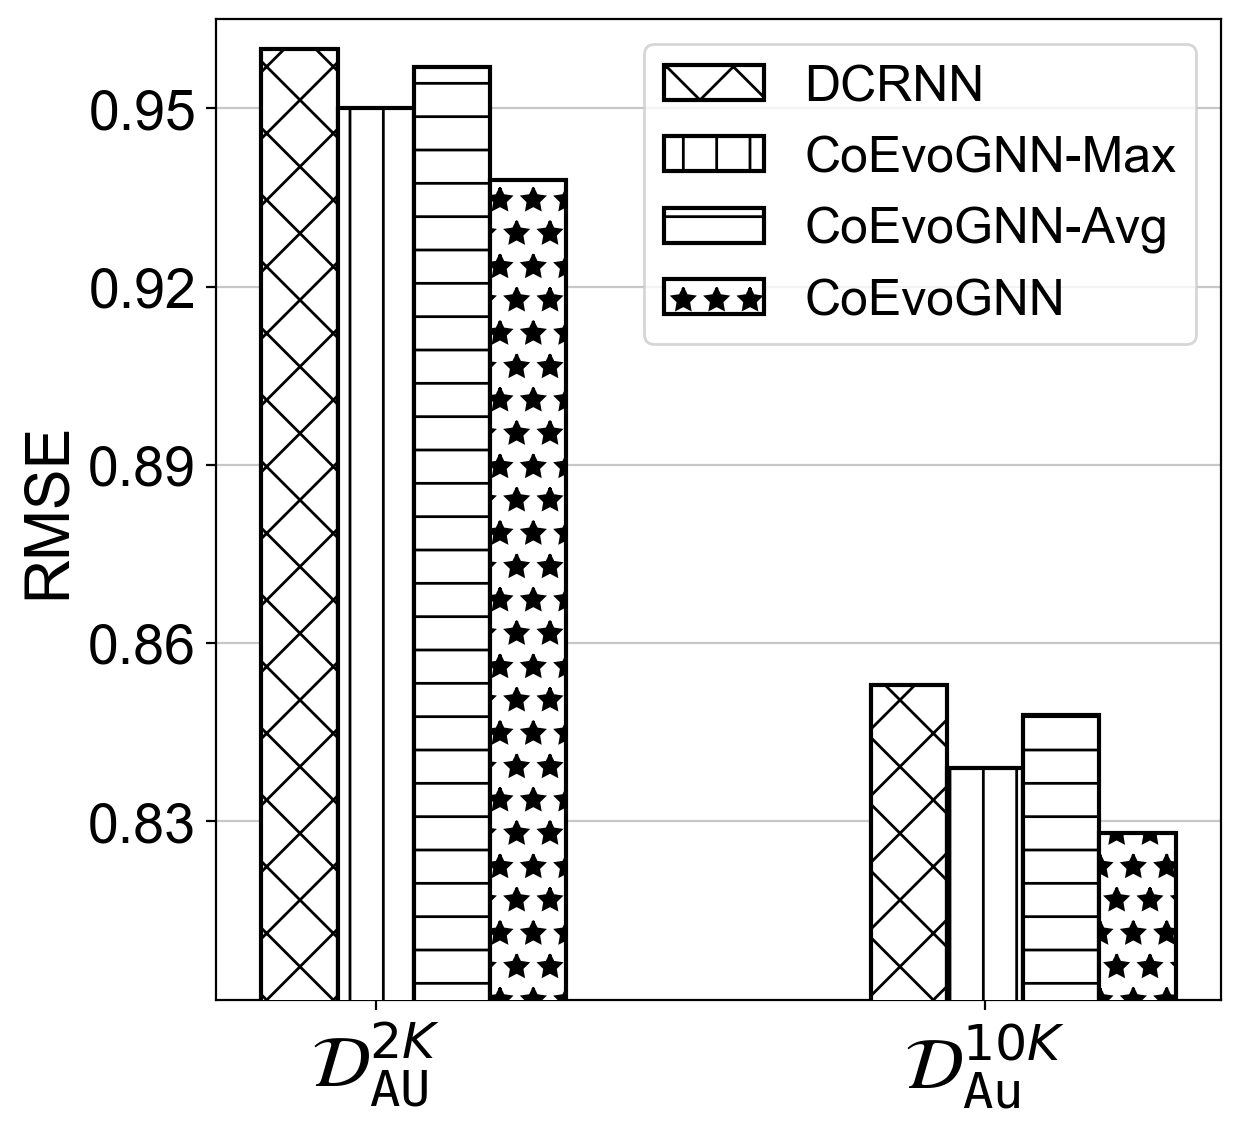}\label{fig:architecture_attention_1}}
	\hfill
	\subfigure[Graph link prediction. Higher F1 indicates better performance.]
    {\includegraphics[width=0.48\linewidth]{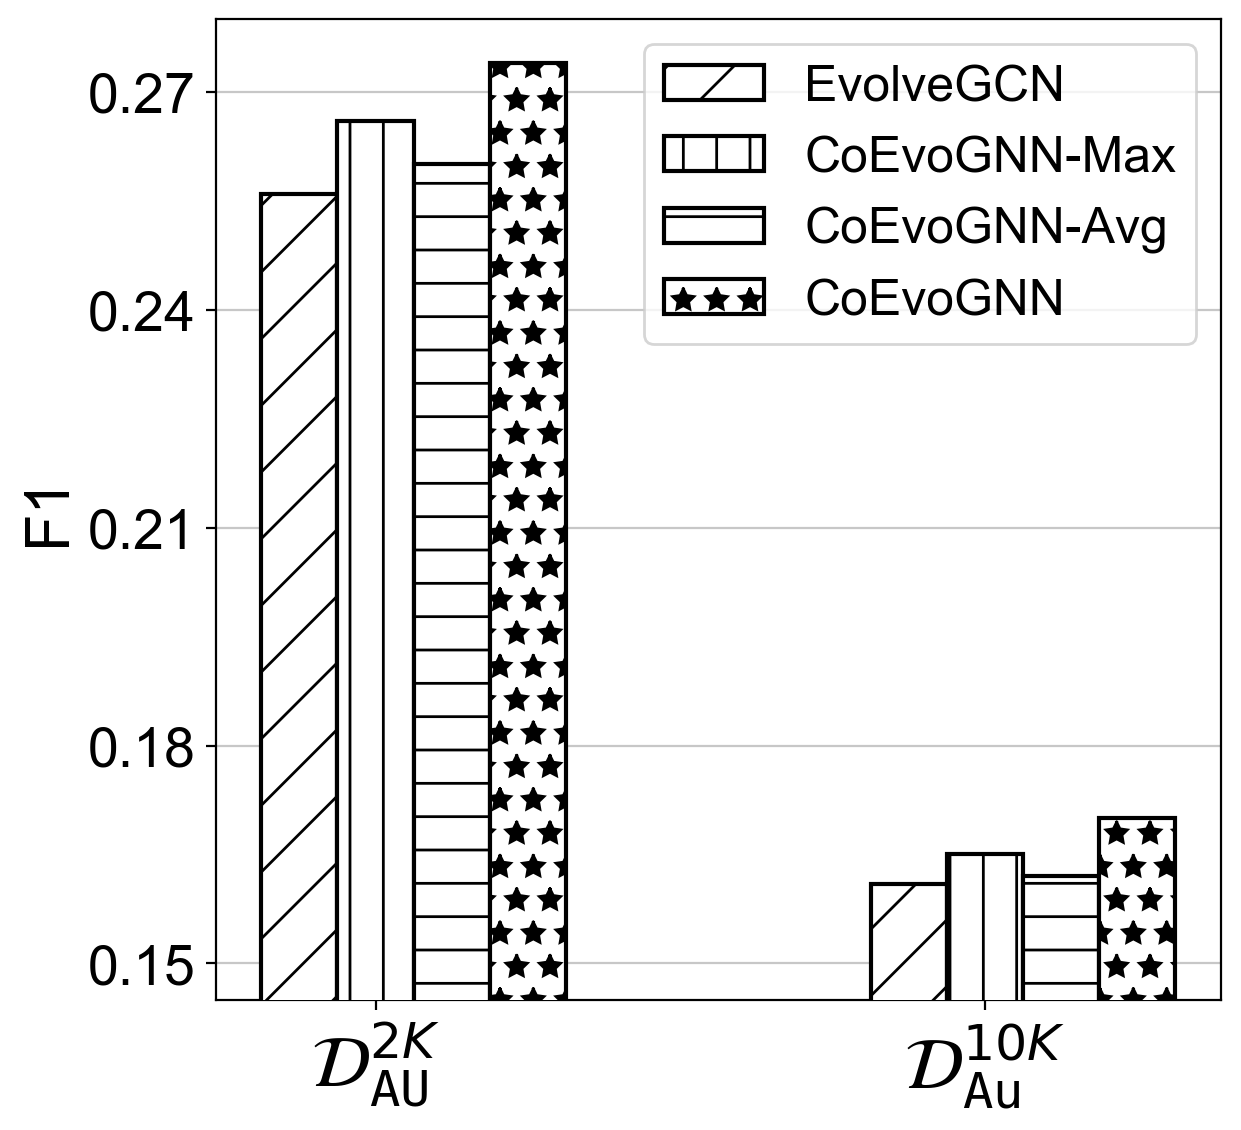}\label{fig:architecture_attention_2}}
	\vspace{-0.2in}
    \caption{Standard \textsc{CoEvoGNN} with self-attention performs better than Max or Avg aggregators.}
    \label{fig:architecture_attention}
    \vspace{-0.2in}
\end{figure}

\begin{table}[t]
	\caption{Forecasting node attributes and links in $\mathcal{D}_{\textsc{au}}^{2K}$ and $\mathcal{D}_{\textsc{au}}^{10K}$ with different values of temporal evolution span $S$.}
	\label{tab:architecture_s}
	\vspace{-0.1in}
	\centering
	
	\scale[0.90]{
	\begin{tabular}{|l|c|c|c|c|}
		\hline
		& \multicolumn{2}{c|}{$\mathcal{D}_{\textsc{au}}^{2K}$} & \multicolumn{2}{c|}{$\mathcal{D}_{\textsc{au}}^{10K}$} \\
		\hline
		 & \multirow{1}*{Attributes} & \multirow{1}*{Links in} & \multirow{1}*{Attributes} & \multirow{1}*{Links in} \\
		 & $\mathbf{X}^{2010}$ & $G^{2010}$ & $\mathbf{X}^{2010}$ & $G^{2010}$ \\
		\hline
		Depth & RMSE & F1 & RMSE & F1 \\
		\hline \hline
		$S=1$		& 0.988 & 0.236 & 0.897 & 0.149 \\
		$S=2$		& 0.952 & 0.259 & 0.863 & 0.162 \\
		$S=3$		& \textbf{0.938} & \textbf{0.274} & 0.832 & \textbf{0.170} \\
		$S=4$		& 0.940 & 0.270 & \textbf{0.828} & \textbf{0.170} \\
		$S=5$		& 0.941 & 0.269 & 0.829 & 0.168 \\
		$S=6$		& 0.941 & 0.271 & 0.830 & 0.167 \\
		$S=7$		& 0.945 & 0.266 & 0.833 & 0.164 \\
		$S=8$		& 0.951 & 0.262 & 0.840 & 0.160 \\
		\hline
	\end{tabular}
	}
	\vspace{-0.15in}
\end{table}

\subsubsection{Contribution of temporal self-attention}
On graph level, \textsc{CoEvoGNN} fuses influence from up to $S$ previous time steps; and, on the node level, it is natural to assume each node have different dependency strengths to its previous states. Another critical aspect of \textsc{CoEvoGNN} is the design of temporal-self-attention (see Line 9 and 12-17 of Algo. \ref{alg:framework}) allowing each node to independently determine the relative importance of previous $S$ snapshots when generating its new embedding. To validate the effectiveness of this design, we build two variants of the model: (1) \textsc{CoEvoGNN-Max} that takes the max pooling operation on node's previous states; and, (2) \textsc{CoEvoGNN-Avg} that takes mean vector of node's previous states (see Line 19 of Algo. \ref{alg:framework}). We compare the improvements of \textsc{CoEvoGNN} and its variants against \textsc{DCRNN} for node attribute prediction, and against \textsc{EvolveGCN} for future graph link prediction. The results are represented in Figure \ref{fig:architecture_attention}.

It is evident that \textsc{CoEvoGNN} significantly outperform the other two variants and producing much lower RMSE values on the task of future node attribute prediction and higher F1 values on the task of graph link prediction. We can also observe that  \textsc{CoEvoGNN-Max} performs slightly better than \textsc{CoEvoGNN-Avg} probably because it is able to extract the most salient latent embeddings from previous states instead of averaging the information. The similar findings on evolutionary virtual currency graphs $\mathcal{D}_{\textsc{bc}}^{\text{otc}}$ and $\mathcal{D}_{\textsc{bc}}^{\text{alp}}$ are not presented here due to space limit. These observations confirm that the design of temporal self-attention over node's previous states is successful in dynamically fusing influence from multiple previous states. Taken together with a reasonable choice of the temporal evolution span $S$, \textsc{CoEvoGNN} is able to model the co-evolution of node attributes and graph structure with self-adapting importance.

\begin{table}[t]
	\caption{Performance of \textsc{CoEvoGNN} on $\mathcal{D}_{\textsc{au}}^{2K}$ and $\mathcal{D}_{\textsc{au}}^{10K}$ with different of training length $T$. Training over time for more years performs better on both tasks.}
	\label{tab:performance_ts}
	\vspace{-0.1in}
	\centering
	
	\scale[0.825]{
	\begin{tabular}{|l|c|c|c|c|}
		\hline
		& \multicolumn{2}{c|}{$\mathcal{D}_{\textsc{au}}^{2K}$} & \multicolumn{2}{c|}{$\mathcal{D}_{\textsc{au}}^{10K}$} \\
		\cline{2-5}
		 & \multirow{1}*{Attributes} & \multirow{1}*{Links in} & \multirow{1}*{Attributes} & \multirow{1}*{Links in} \\
		 & $\mathbf{X}^{2010}$ & $G^{2010}$ & $\mathbf{X}^{2010}$ & $G^{2010}$ \\
		\hline
		Training & RMSE & F1 & RMSE & F1 \\
		\hline \hline
		$01-09$		& 0.938 & \textbf{0.274} & \textbf{0.828} & \textbf{0.170} \\
		$02-09$		& \textbf{0.937} & 0.266 & 0.845 & 0.158 \\
		$03-09$		& 0.943 & 0.258 & 0.846 & 0.145 \\
		$04-09$		& 0.954 & 0.249 & 0.860 & 0.138 \\
		$05-09$		& 0.958 & 0.230 & 0.883 & 0.121 \\
		$06-09$		& 0.961 & 0.211 & 0.896 & 0.105 \\
		$07-09$		& 0.972 & 0.182 & 0.912 & 0.087 \\
		$08-09$		& 1.054 & 0.169 & 0.945 & 0.078 \\
		\hline
	\end{tabular}
	}
	\vspace{-0.1in}
\end{table}

\begin{figure}[t]
    \centering
    \subfigure[Training time of \textsc{CoEvoGNN} is linear to the training graph sequence length $T$.]
    {\includegraphics[width=0.48\linewidth]{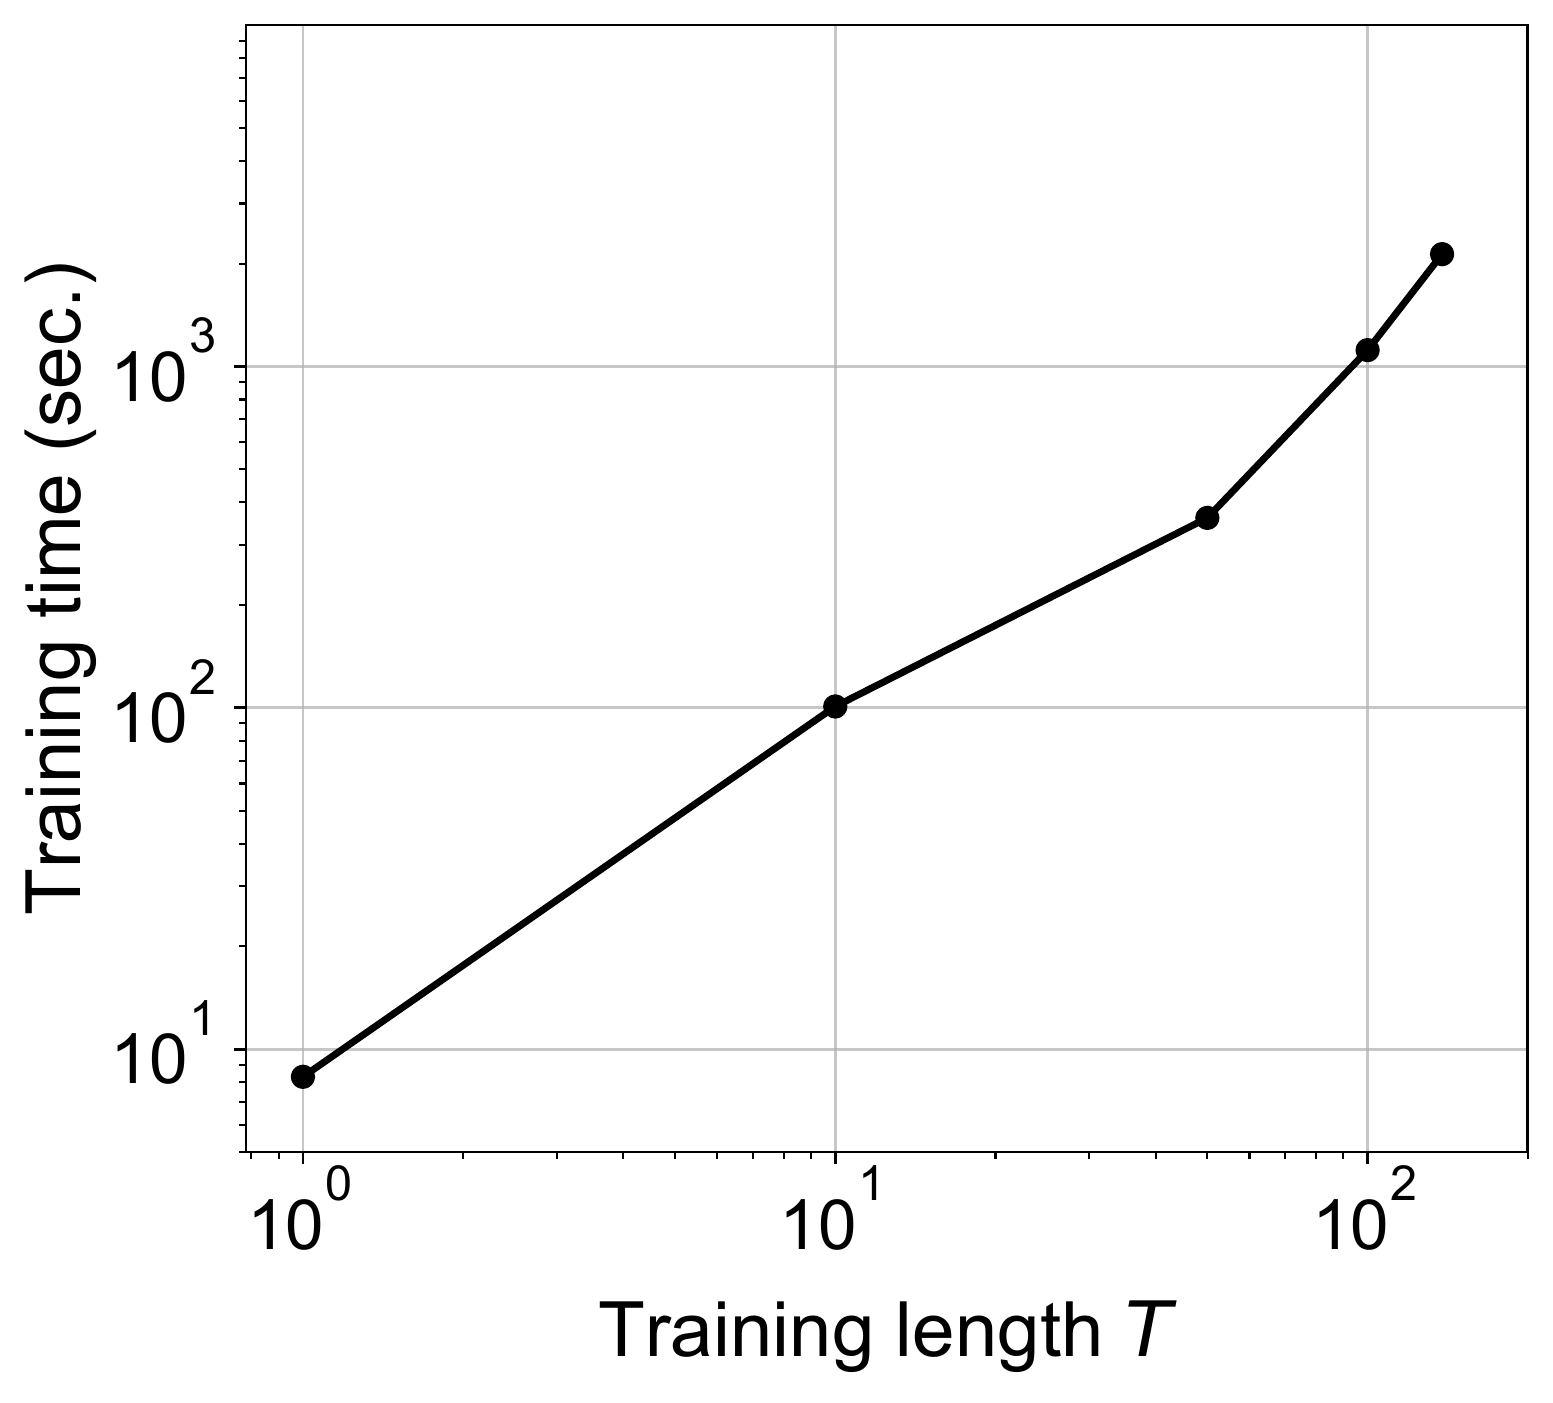}\label{fig:efficiency_t}}
    \hfill
    \subfigure[Training time of \textsc{CoEvoGNN} is insensitive to the temporal evolution span $S$.]
    {\includegraphics[width=0.48\linewidth]{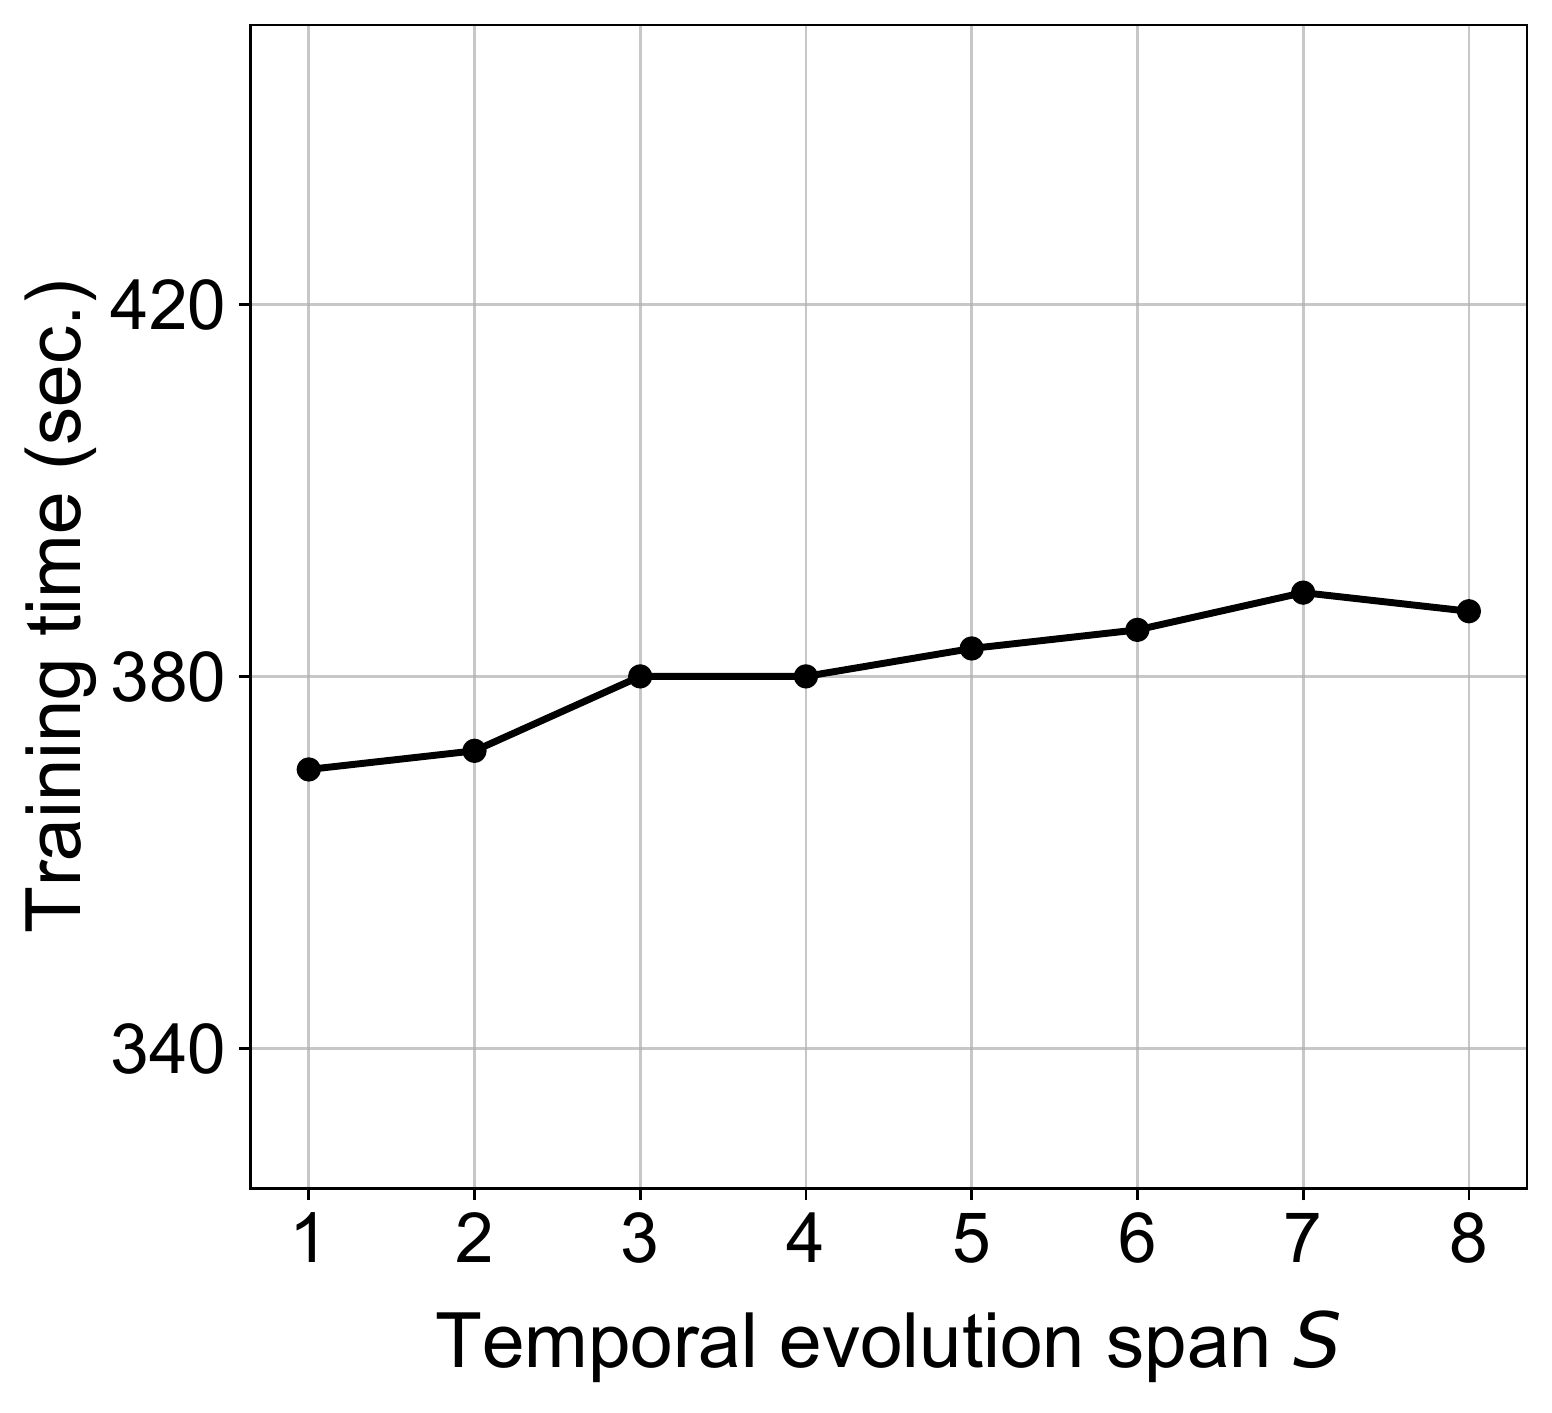}\label{fig:efficiency_s}}
	\vspace{-0.2in}
    \caption{Effiency of \textsc{CoEvoGNN} on $\mathcal{D}_{\textsc{bc}}^{\text{alp}}$ with different values of training length $T$ and temporal evolution span $S$.}
    \label{fig:efficiency}
    \vspace{-0.1in}
\end{figure}

\subsection{Effect of training length $T$}
Since \textsc{CoEvoGNN} generates node embeddings along the training time steps, we examine the effect of the training length $T$ on the performance of \textsc{CoEvoGNN}. Specifically, we vary the number of graphs in the training sequence from all historical graphs to the only one before the test graph. Table \ref{tab:performance_ts} presents the results on evolutionary co-authorship graphs $\mathcal{D}_{\textsc{au}}^{2K}$ and $\mathcal{D}_{\textsc{au}}^{10K}$. 

On dataset $\mathcal{D}_{\textsc{au}}^{2K}$, \textsc{CoEvoGNN} achieves the best performance for predicting graph links in $G^{2010}$ when using all historical graph snapshots from $2001$ to $2009$; and has comparable good performance for predicting node attribute in $\mathbf{X}^{2010}$ if being fed graph snapshots starting from $2002$. The trend is consistent on the $\mathcal{D}_{\textsc{au}}^{10K}$ dataset: \textsc{CoEvoGNN} achieves its best performance for both tasks when trained using all historical graph snapshots. This indicates that longer training ranges lead to better performance of \textsc{CoEvoGNN}, which follows our intuition that longer training range provides more information and can make the model yeild better performance.

\subsection{Efficiency and sensitivity}
\label{sec:sensitivity}
We test the time efficiency of \textsc{CoEvoGNN} through different values of training length $T$ and temporal evolution span $S$. All experiments are conducted on single server with dual 12-core Intel Xeon 2.10GHz CPUs with single NVIDIA GeForce GTX 2080 Ti GPU. Figure \ref{fig:efficiency} shows the model's per epoch training time is generally linear to the length of the training graph sequence and is insensitive to different values of temporal evolution span. This is also confirmed by our analysis on the complexity of \textsc{CoEvoGNN} given in Section \ref{subsec:complexity}.

%We also investigate the hyperparameter $\alpha$ of \textsc{CoEvoGNN} for balancing the attribute and structure evolutionary losses. Empirical analysis shows that the model is able to achieve optimal performance when setting $\alpha$ to mix those two evolutionary losses differing by no more than one order of magnitude.
